# Supplementary material for: Causal Inference Struggles with Agency on Online Platforms
Source: arXiv:2107.08995 source file (2022-05-10)
Supplement: Supplementary file 1 [file appendix.tex]

\appendix

\section{Balance in IPTW} \label{app:balance}
In IPTW, the treatment-unexposed and treatment-exposed groups are supposed have the same distribution of covariates after weighting. The following figures show the absolute standardized difference between the mean of covariates before and after weighting in all four cases. Achieving perfect balance is generally unattainable in practice, and there is no single accepted heuristic for assessing balance, but generally a difference of less than 0.1 has been accepted as reasonably balanced ~\citep{austin2015moving}. In all cases, weighting appears to generally balance the covariates.

\begin{figure}[h]
    \centering
    \includegraphics[width=\textwidth]{figures/mr_push_balance.pdf}
    \label{fig:mr_push_balance}
\end{figure}

\begin{figure}[h]
    \centering
    \includegraphics[width=\textwidth]{figures/mr_email_balance.pdf}
    \label{fig:mr_email_balance}
\end{figure}

\begin{figure}[h]
    \centering
    \includegraphics[width=\textwidth]{figures/timeline_balance.pdf}
    \label{fig:timeline_balance}
\end{figure}

\begin{figure}[h]
    \centering
    \includegraphics[width=\textwidth]{figures/toxicity_balance.pdf}
    \label{fig:toxicity_balance}
\end{figure}
